# Supplementary material for: Free-rider Attacks on Model Aggregation in Federated Learning
Source: arXiv:2006.11901 source file (2021-02-22)
Supplement: Supplementary file 1 [file old_supplementary.tex]

\section{Complete Proofs}

\subsection{Proof of Theorem \ref{deterministic_theorem}}
\label{deterministic_proof}

\begin{proof}\label{proof:plain}
	The aggregation at the server level follows:
	\begin{align}
	\label{eq:aggregation_plain}
	\theta^{t+1}
	=\sum_{j\in J}\frac{M_j}{N} \tilde{\theta}_j^{t+1} + \frac{M_K}{N} \tilde{\theta}^t.
	\end{align}
	\noindent By considering a continuous increment of time and according to the noise process hypothesis of Section \ref{free-rider_strategies} we obtain the following first order stochastic differential equation:
%	\begin{align}
%	\dot\tilde{\theta}^t
%	=\sum_{j\in J}\frac{M_j}{N}\tilde{\theta}_j(t)+\beta\tilde{\theta}^t,
%	\end{align}
	\begin{align}
	\mathrm{d}\tilde{\theta}^t
	&=-\beta \sum_{j\in J} \frac{M_j}{ N - M_k } [ \mathrm{d} \E{\hat{\theta}_j^t} + (1-\epsilon) \E{\hat{\theta}_j^t} \mathrm{d}t ] \nonumber\\
	&-\beta\sum_{j\in J}\frac{M_j}{N-M_k} \rho_j\mathrm{d}W_{t_j} + \beta(1-\epsilon)\tilde{\theta}^t\mathrm{d}t.
	\end{align}
%	\noindent where we define $\beta=\frac{M_K}{N}-1$. According to the noise process hypothesis of Section (\ref{free-rider_strategies}), we thus obtain the stochastic differential equation:
%	\begin{align}
%	\mathrm{d}\tilde{\theta}^t = \left(\beta \tilde{\theta}^t + \sum_{j\in J}\frac{M_j}{N}{\theta}_j(t)\right)\mathrm{d}t  + \sum_{j\in J}\left(\frac{M_j}{N} (1+\beta)\eta \mathrm{d}W^1_j(t) + \frac{M_j}{N} \rho_j \mathrm{d}W^2_j(t) \right),
%	\label{eq:plain_sde}
%	\end{align}
	which can be rewritten as 
	\begin{align}
	\label{eq:equa_diff_theo_1}
	\mathrm{d}\left(e^{-\mu t}\tilde{\theta}^t\right)
	&=-\beta e^{-\mu t}[e^{-\nu t}\sum_{j\in J}\frac{M_j}{N-M_k}\mathrm{d}\left(e^{\nu t}\E{ \hat{\theta}_j^t }\right)\nonumber\\
	&-\sum_{j\in J}\frac{M_j}{N-M_k} \rho_j\mathrm{d}W_{t_j} ].
	\end{align}
	where $\mu=\beta(1-\epsilon)$ and $\nu=1-\epsilon$. For each client, $\eta_j$ is positive and inferior to 1 by definition of the exponential function and under the quadratic approximation of the local loss function in Section \ref{sec:sgd_perturbation}. Thus $\epsilon\in ]0,1[$ which implies that $\mu<0$ and $\nu>0$.
	
	The associated solution of equation (\ref{eq:equa_diff_theo_1}):
% 	\begin{equation}
% 	d[e^{-\beta t}\tilde{\theta}^t]
% 	=[e^{-\beta t}\ \dot\tilde{\theta}^t-\beta\ e^{-\beta t}\ \tilde{\theta}^t]dt
% 	=\sum_{j\in J}\frac{M_j}{N}\ e^{-\beta t}\ \theta_j(t)dt+\frac{M_J}{N}\eta dW_t
% 	\end{equation}
% 	\begin{equation}
% 	[e^{-\beta t}\tilde{\theta}^t]_{t_0}^t
% 	=\sum_{j\in J}\frac{M_j}{N}\int_{t_0}^te^{-\beta x}\ \theta_j(x)\ dx
% 	+\int_{t_0}^te^{-\beta x}\frac{M_J}{N}\eta dW_x
% 	\end{equation}
	\begin{align}
	\label{equa_dif_solved}
	\tilde{\theta}^t
	&= e^{\mu t}[c_0-\beta\sum_{j\in J}\frac{M_j}{N-M_K}\underbrace{\int_{t_0}^t e^{-(\mu+\nu) x}\ \mathrm{d}\left(e^{\nu t}\E{ \hat{\theta}_j^t }\right)}_\text{\textbf{A}}\nonumber\\
	&-\beta\sum_{j\in J}\frac{M_j}{N-M_K} \underbrace{\int_{t_0}^t \rho_j e^{ - \mu  x} \mathrm{d} {W_{j}}_x}_\text{\textbf{B}} ],
%	& + \sum_{j\in J}\frac{M_j}{N} \rho_j \underbrace{\int_{t_0}^t e^{-\beta x}d{W_j^2}_x}_\text{\textbf{B2}}],
	\end{align}
%	\begin{align}
%	\label{equa_dif_solved}
%	\tilde{\theta}^t
%	&= e^{\beta t}[c_0+\sum_{j\in J}\frac{M_j}{N}\underbrace{\int_{t_0}^t e^{-\beta x}\ \theta_j(x)dx}_\text{\textbf{A}}\nonumber\\
%	&+\sum_{j\in J}\frac{M_j}{N} (1+\beta)\eta \underbrace{\int_{t_0}^t e^{-\beta x}d{W_j^1}_x}_\text{\textbf{B1}} \nonumber\\
%	& + \sum_{j\in J}\frac{M_j}{N} \rho_j \underbrace{\int_{t_0}^t e^{-\beta x}d{W_j^2}_x}_\text{\textbf{B2}}],
%	\end{align}
	where we denote $c_0=e^{-\mu t_0}\tilde{\theta}^{t_0}$. In the following part of the proof we study the asymptotic properties of solution ($\ref{equa_dif_solved}$) separately.
	\begin{itemize}
	
		\item \textbf{Asymptotic convergence of A}.
		We study the asymptotic properties of (A) by first integrating by parts the integrals $\int_{t_0}^te^{-(\mu +\nu) x}\ \mathrm{d}(e^{\nu x}\E{ \hat{\theta}_j^x })$:
		\begin{align}
%		\label{IPP_equa_diff}
		\int_{t_0}^te^{-(\mu+\nu) x} \mathrm{d}(e^{\nu x}\E{ \hat{\theta}_j^x })
		&=[e^{-\mu x}\E{ \hat{\theta}_j^x }]_{t_0}^t\nonumber\\
		&+(\mu+\nu)\int_{t_0}^t e^{-\mu x} \E{ \hat{\theta}_j^x } dx,\nonumber\\
%		&= -\frac{1}{\beta}e^{-\beta t}\theta_j(t)+ \frac{1}{\beta} \int_{t_0}^t e^{-\beta x} \dot\theta_j(x) dx + C.
		\end{align} 
		Doing another integration by parts on the integral $\int_{t_0}^t e^{-\mu x} \E{ \hat{\theta}_j^x } dx$ gives
		\begin{align}
		\int_{t_0}^t e^{-\mu x} \E{ \hat{\theta}_j^x } dx
		&=[\frac{1}{-\mu}e^{-\mu x}\E{ \hat{\theta}_j^x }]_{t_0}^t\nonumber\\
		&+\frac{1}{\mu}\int_{t_0}^t e^{-\mu x} \frac{\mathrm{d}\E{ \hat{\theta}_j^x }}{\mathrm{d}x} \mathrm{d}x,\nonumber\\
%		&= -\frac{1}{\mu}e^{-\mu t}\theta_j(t)+ \frac{1}{\mu} \int_{t_0}^t e^{-\mu x} \frac{\mathrm{d}\E{ \hat{\theta}_j^x }}{\mathrm{d}x} dx + C.
		\end{align} 
		leading to
		\begin{align}
		\label{IPP_equa_diff}
		\int_{t_0}^te^{-(\mu+\nu) x} \mathrm{d}(e^{\nu x}\E{ \hat{\theta}_j^x })
		&=-\frac{\nu}{\mu}e^{-\mu t}\E{ \hat{\theta}_j^t }\nonumber\\
		&+(1+\frac{\nu}{\mu})\int_{t_0}^t e^{-\mu x} \frac{\mathrm{d}\E{ \hat{\theta}_j^x }}{\mathrm{d}x}\mathrm{d}x.\nonumber\\
		%		&= -\frac{1}{\beta}e^{-\beta t}\theta_j(t)+ \frac{1}{\beta} \int_{t_0}^t e^{-\beta x} \dot\theta_j(x) dx + C.
		\end{align} 
		To investigate the asymptotic properties of the combination of the integrals (\ref{IPP_equa_diff}) in equation (\ref{equa_dif_solved}), we first note that $\beta\frac{\nu}{\mu} = 1$. We can therefore study the limit $t\rightarrow\infty$ of the quantity:
		\begin{align}
		 g(t) &=\sum_{j\in J}\dfrac{M_j}{M_K-N}e^{\mu t}\int_{t_0}^t e^{-\mu x}\ \frac{\mathrm{d}\E{ \hat{\theta}_j^x }}{\mathrm{d}x}\ dx.
		\end{align}
		We assume smooth convergence for the expected model $\E{ \hat{\theta}_j^t }$ under the condition $|\frac{\mathrm{d}\E{ \hat{\theta}_j^t }}{\mathrm{d}t}|=O({t^{-\alpha_j}})$, i.e.   $\exists\ t_j,R_i\in \mathbb{R}^+\ \text{such that}\ \forall t\ge t_j, |\frac{\mathrm{d}\E{ \hat{\theta}_j^t }}{\mathrm{d}t}|\le\frac{R_i}{t^{\alpha_j}}$. By considering $t_0=\max_{j\in J}(t_j)$, $\alpha=\min_{j\in J}(\alpha_j)$ and $t>t_0$, the triangular inequality gives:
		\begin{align}
		|g(t)|
		&\le \sum_{j\in J}\dfrac{M_j}{M_K-N}e^{\mu t}|\int_{t_0}^t e^{-\mu x} \frac{\mathrm{d}\E{ \hat{\theta}_j^x }}{\mathrm{d}x}\ dx|,
		\end{align}
		and for the assumption of piece-wise continuity of  $\frac{\mathrm{d}\E{ \hat{\theta}_j^t }}{\mathrm{d}t}$ in $[t_0,t]$ we get:
		\begin{align}
		|g(t)|
		&\le \sum_{j\in J}\dfrac{M_j}{N-M_K}e^{\mu t}\int_{t_0}^t e^{-\mu x} |\frac{\mathrm{d}\E{ \hat{\theta}_j^x }}{\mathrm{d}x}| dx \nonumber\\
		&\le\sum_{j\in J}\dfrac{M_j}{N-M_K}R_ie^{\mu t}\int_{t_0}^t \frac{e^{-\mu x}}{x^\alpha}  dx.
		\end{align}
	% 	\begin{equation}
	% 	|g(t)|
	% 	\le \sum_{j\in J}\dfrac{M_j}{N-M_K}R_ie^{\beta t}\int_{t_0}^t \frac{e^{-\beta x}}{x^\alpha} dx
	% 	\end{equation}
		Considering that $\lim_{t\rightarrow+\infty}e^{-\mu t}=\lim_{t\rightarrow+\infty}\int_{t_0}^{t}\frac{e^{-\mu x}}{x^\alpha}\mathrm{d}x=+\infty$ and $\forall t\in \mathbb{R},\ \frac{\mathrm{d}e^{-\mu t}}{\mathrm{d}t}>0$, by using L'H\^{o}pital's rule, we get:
%		Since that $\alpha>0$, $t_0>0$, $-\beta>0$, and $\epsilon\in[0,1[$ lemma  in Proposition \ref{exponential_integral} shows that %with $k=-\beta$ and get that 
		\begin{align}
		   |g(t)|&\leq e^{\mu t}\int_{t_0}^t \frac{e^{-\mu x}}{x^\alpha}\  dx\xrightarrow{t\rightarrow+\infty}0.
		\end{align}
	
	
	\item \textbf{Asymptotic convergence of B}.
	The asymptotic properties of the stochastic integral B follow from the general properties of Ito's integrals. For any constant $L$, we have:
	\begin{align}
	    \E{L e^{\mu t}  \int_{t_0}^t e^{-\mu x} dW_x} &= 0, \label{Ito_exp}\\
	    \VAR{L e^{\mu t} \int_{t_0}^t e^{-\mu x} dW_x} & = L^2 e^{2 \mu t} \int_{t_0}^t e^{-2\mu x} dW_x \label{Ito_var}\\
	    & = - \frac{L^2 e^{2 \mu t}}{2\mu}  (e^{-2\mu t} -e^{-2\mu t_0}) \\
	    &\xrightarrow{t\rightarrow+\infty} - \frac{L^2}{2\mu},
	\end{align}
	where the first equality in line ($\ref{Ito_var}$) is due to Ito's isometry.
	\end{itemize}
	%So $|g(t)| \xrightarrow{t\rightarrow+\infty}0$\\
% 	In addition, if we use Appendix \ref{sec:theta_j_noise}, with $k=-\beta$ and $c=\frac{M_j}{N}\eta=-\beta\eta$, we get that:
% 	\begin{equation}
% 	    \E{e^{\beta t}\int_{t_0}^te^{-\beta x}\frac{M_j}{N}\eta dW_x}
% 	    \xrightarrow{t\rightarrow+\infty}0
% 	    \text{ and }
% 	    \VAR{e^{\beta t}\int_{t_0}^te^{-\beta x}\frac{M_j}{N}\eta dW_x}
% 	    \xrightarrow{t\rightarrow+\infty}\frac{-\beta}{2}\eta^2
% 	\end{equation}
	By substituting in equation (\ref{equa_dif_solved}) the convergence results for the quantities (\ref{IPP_equa_diff}), (\ref{Ito_exp}) and (\ref{Ito_var}), we finally conclude that: 
	\begin{align}
	    \E{\tilde{\theta}^t}
	    &\xrightarrow{t\rightarrow+\infty} \sum_{j\in J}\frac{M_j}{N-M_K}\E{ \hat{\theta}_j^t },\\
	    %
	    \VAR{\tilde{\theta}^t}
	    &\xrightarrow{t\rightarrow+\infty} -\frac{\beta^2}{2\mu}\sum_{j\in J} \left( \frac{M_j}{ N - M_K } \right)^2 \rho_j^2 \\
	    &=-\frac{\beta}{2(1-\epsilon)}\sum_{j\in J} \left( \frac{M_j}{ N - M_K } \right)^2 \rho_j^2.
	\end{align} 
	
	Note: in the special case $\beta=0$, then equation (\ref{eq:aggregation_plain}) can be expressed as $\tilde{\theta}^{t+1} = \tilde{\theta}^t $ thus $\tilde{\theta}^t=\theta^0$.
	    
	
	
	
	
	
	
\end{proof}

\subsection{Proof of Theorem \ref{theo:noise_additive}}
\label{stochastic_proof_additive}


\begin{proof} 
    The differential equation governing the disguised attack is
    \begin{align}
    \mathrm{d}\tilde{\theta}^t
    &=-\beta\sum_{j\in J}\frac{M_j}{N-M_k}[\mathrm{d}\E{ \hat{\theta}_j^t }+(1-\epsilon)\E{ \hat{\theta}_j^t }\mathrm{d}t]\nonumber\\
    &-\beta\sum_{j\in J}\frac{M_j}{N-M_k} \rho_j \mathrm{d}W_{t_j} \nonumber\\
    &+ \beta ( 1 - \epsilon ) \tilde{\theta}^t \mathrm{d}t + (\beta + 1 ) \varphi(t) \mathrm{d}W_t.
    \end{align}
%    
%    \begin{align}
%    \mathrm{d}\tilde{\theta}^t & = \left(\beta \tilde{\theta}^t + \sum_{j\in J}\frac{M_j}{N}{\theta}_j(t)\right)\mathrm{d}t \nonumber\\
%    &+ \sum_{j\in J}\left(\frac{M_j}{N} (1+\beta)\eta \mathrm{d}Wt^1_j + \frac{M_j}{N} \rho_j \mathrm{d}Wt^2_j \right) \nonumber \\ 
%    &+ \frac{M_K}{N} \varphi(t) \mathrm{d}Wt. 
%    \label{eq:add_sde}
%    \end{align}
    We note that this equation differs from the one in proof (\ref{proof:plain}) for the last term only. We derive conditions for the perturbation $\varphi(t)>0$ for ensuring convergence, by studying the integral
    \begin{align}
    \mathcal{L}(t) & = (1+\beta)e^{\mu t}\int_{t_0}^t \varphi(x) e^{-\mu x} dW_x.
    \end{align}
    We prove the convergence of $\mathcal{L}(t)$ when $\varphi(t) = \varphi$. Considering the work done in prof (\ref{proof:plain}), we thus have  
     \begin{align}
 	    \E{\mathcal{L}(t)}
 	    &\xrightarrow{t\rightarrow+\infty} 0, \\
 	    \text{and }\VAR{\mathcal{L}(t)} 
 	    &\xrightarrow{t\rightarrow+\infty} -\frac{(1+\beta)}{2\beta(1-\epsilon)}\varphi^2.
 	   \end{align}



	
	
	
	
\end{proof}

\subsection{Proof of Corollary \ref{cor:noise_additive_multi}}
\begin{proof}
The differential equation governing the disguised attack for many free-riders:
\begin{align}
\mathrm{d}\tilde{\theta}^t
&=-\beta\sum_{j\in J}\frac{M_j}{N-M_k}[\mathrm{d}\E{ \hat{\theta}_j^t }+(1-\epsilon)\E{ \hat{\theta}_j^t }\mathrm{d}t]\nonumber\\
&-\beta\sum_{j\in J}\frac{M_j}{N-M_k} \rho_j \mathrm{d}W_{t_j}  \nonumber\\
&+ \beta (1-\epsilon) \tilde{\theta}^t\mathrm{d}t + \sum_{k\in K}\frac{M_k}{N}\varphi_k(t) \mathrm{d}W_{t_k}.
\end{align}
We note that this equation differs from the one in proof (\ref{proof:plain}) for the last term only. Since proof (\ref{stochastic_proof_additive}) already proves the convergence for a single term $\mathcal{L}_k(t) = \frac{M_k}{N}e^{\mu t}\int_{t_0}^t \varphi_k(x) e^{-\mu x} dW_x.$ when $\varphi_k(t) = \varphi_k$. The corollary thus follows from the linearity of the last term:
\begin{align}
    \E{\sum_{k\in K}\Lcal_k(t)}&=0,\\
    \text{ and }
    \VAR{\sum_{k\in K}\Lcal_k(t)}&\xrightarrow{t\rightarrow+\infty}  -\sum_{k\in K}\frac{M_k^2}{N^2}\frac{\varphi_k^2}{2\beta(1-\epsilon)}.
\end{align} 

%Note: when $\beta=0$, equation (\ref{eq:add_sde_many}) can be expressed as $\mathrm{d}\tilde{\theta}^t =\sum_{k\in K}\frac{M_k}{N} \varphi_k(t) \mathrm{d}Wt_k$ thus for all $\gamma_k>1$, $\E{\tilde{\theta}^t}=\theta_0(t)$ and $\VAR{\tilde{\theta}^t}=0$.

\end{proof}










\subsection{Proof of Corollary \ref{cor:fair_decay_noise}}

\begin{proof}
The differential equation the disguised attack is
\begin{align}
\mathrm{d}\tilde{\theta}^t
&=-\beta\sum_{j\in J}\frac{M_j}{N-M_k}[\mathrm{d}\E{ \hat{\theta}_j^t }+(1-\epsilon)\E{ \hat{\theta}_j^t }\mathrm{d}t]\nonumber\\
&-\beta\sum_{j\in J}\frac{M_j}{N-M_k} \rho_j(t) \mathrm{d}W_{t_j}^2 \nonumber\\
&+ \beta(1-\epsilon)\tilde{\theta}^t\mathrm{d}t+ (\beta+1)\varphi(t) \mathrm{d}W_{t_k}.
\end{align}
We consider $\rho_j(t)=\rho_j +O(t^{-a_j})$ and $\varphi(t)=\varphi+O(t^{-a})$ with $a_j>0$  and $a>0$ for $t>t_0>0$. We can note that this equation differs from the one in proof (\ref{proof:plain}) by the time varying contribution of $\rho_j(t)$ and $\varphi_k(t)$. We derive conditions for the perturbation $\varphi(t)$ and $\rho_j(t)$ for ensuring convergence by studying the integral 
\begin{equation}
	\Lcal(f,t)=Ae^{\mu t}\int_{t_0}^{t}f(x)e^{-\mu x}\mathrm{d}x,
\end{equation}
where $A$ is constant and $f(t)=O(t^{-\gamma})$, $\gamma>0$. In particular, let $\sigma>0$ and $t_0>0$ such that $f(t)\le\sigma t^{-\gamma}$. We thus have $\Lcal(f,t)\le\Lcal'(f,t)=A\sigma e^{\mu t}\int_{t_0}^{t}\frac{e^{-\mu x}}{x^{\gamma}}\mathrm{d}W_x$, and 
%We show in proof (\ref{stochastic_proof_additive}) that for $\Lcal_{\rho_j}(t)=\frac{M_j}{N}e^{\beta t}\int_{t_0}^t \rho_j(t)e^{-\beta x}d{W_j^2}_x$, we have:
\begin{align}
\E{\Lcal'(f,t)}
\xrightarrow{t\rightarrow+\infty}0
\text{ and }
\VAR{\Lcal'(f,t)}
\xrightarrow{t\rightarrow+\infty}0,
\end{align}
where the limit of the variance is due to Ito's isometry and L'H\^{o}pital's rule.

Consequently, the time-varying contribution in $\rho_j(t)$ and $\varphi(t)$ does not change the asymptotic variance. Thus, Theorem \ref{deterministic_theorem}, Theorem \ref{theo:noise_additive}, and Corollary \ref{cor:noise_additive_multi} have the same asymptotic behaviours with $\rho_j(t)=\rho_j +O(t^{-a_j})$ and $\varphi(t)=\varphi+O(t^{-a})$ as with $\rho_j(t)=\rho_j$ and $\varphi(t)=\varphi$.
%Thus for Theorem \ref{deterministic_theorem} and \ref{theo:noise_additive} and for Corollary \ref{cor:noise_additive_multi}, the asymptotic convergence of $\tilde{\theta}^t$ follows:
%\begin{align}
%    \E{\tilde{\theta}^t}
%    &\xrightarrow{t\rightarrow+\infty} \sum_{j\in J}\frac{M_j}{N-M_K}\theta_j(t),\\
%    \VAR{\tilde{\theta}^t}
%    &\xrightarrow{t\rightarrow+\infty} -\frac{1}{2\beta}\sum_{j\in J} (\frac{M_j}{N})^2 (1+\beta)^2\eta^2  \\
%    & = -\frac{(1+\beta)^2\eta^2 }{2\beta}\sum_{j\in J} (\frac{M_j}{N})^2  \\
%    & = \frac{(N - \sum_j M_j)^2\eta^2}{2N^2}\frac{N}{\sum_j M_j} \sum_j (\frac{M_j}{N})^2\\
%    & = \frac{(N - \sum_j M_j)^2\eta^2}{2N^2}\frac{1}{\sum_j \frac{M_j}{N}} \sum_j (\frac{M_j}{N})^2.
%\end{align}  

%Note: Considering $\rho_j(t)$ instead of $\rho_j$ for the special case $\beta=0$ does not change the reformulation of equation (\ref{eq:aggregation_plain}), equation (\ref{eq:add_sde}), and equation (\ref{eq:add_sde_many}) seen for the special case $\beta=0$ in Theorem \ref{deterministic_theorem}, Theorem \ref{theo:noise_additive}, and Corollary \ref{cor:fair_decay_noise}. 

\end{proof}
